# Supplementary material for: Avalanches and Structural Change in Cyclically Sheared Silica Glass
Source: arXiv:2108.07469 ancillary file (2021-08-17)
Supplement: Supplementary file 1 [file SM_silica_structure.pdf]

# Supplemental Material for
# "Avalanches and Structural Change in Cyclically Sheared Silica Glass"

Himangsu Bhaumik,[1] Giuseppe Foffi,[2] and Srikanth Sastry[1,*]

[1] *Jawaharlal Nehru Center for Advanced Scientific Research, Jakkur Campus, Bengaluru 560064, India.*
[2] *Université Paris-Saclay, CNRS, Laboratoire de Physique des Solides, 91405 Orsay, France*

## S-1. MODEL: MODIFIED BKS SILICA

The modified BKS potential [1] of silica proposed by Voivod *et al.* [2] is given by

$$U(r_{ij}) = \frac{1}{4\pi\epsilon_0}\frac{q_i q_j}{r_{ij}} + \begin{cases} A_{ij}e^{-B_{ij}r_{ij}} - C_{ij}r_{ij}^{-6} + \phi(r_{ij}), & r_{ij} \le r_s \\ \sum_{k=3}^{5} D_{ij}^k (r_{ij} - R_c)^k, & r_s < r_{ij} < r_c \\ 0, & r_{ij} \ge r_c \end{cases} \quad \text{(S1)}$$

where, the short-range term $\phi(r_{ij}) = 4\epsilon_{ij}[(\sigma_{ij}/r_{ij})^{30} - (\sigma_{ij}/r_{ij})^6]$ is added for $r < r_s$ to prevent a negative divergence that could result in the fusion of some atoms. The Coulomb term is evaluated by Ewald summation with an Ewald parameter $\alpha = 2.5\mathring{A}^{-1}$. The momentum space summation is carried out to a radius of six reciprocal lattice points. The real space part of the potential is truncated at $r_s = 7.7747\mathring{A}$. For $r_s < r < r_c$, with $r_c = 10\mathring{A}$, a fifth order polynomial is added to make the potential goes to zero smoothly. The coefficients of $\phi(r_{ij})$ are chosen such that the modified BKS potential has no inflection at small $r$. The values of all the parameters of the potential can be found in Ref. 2.

## S-2. ENERGY EVOLUTION

The evolution of the potential energy per atom measured for stroboscopic configurations ($\gamma = 0$) under athermal quasistatic (AQS) shear protocol is shown in Figs. S1(a) and S1(c) as a function of accumulated strain $\gamma_{acc} = 4\gamma_{max}n_{cycle}$ (where $n_{cycle}$ is the number of cycles) for $T = 2500K$ and $T = 6000K$, respectively. In each case, the starting configurations are local energy minimum structures (inherent structures) obtained from instantaneous quenches of sample equilibrium liquid configurations at the respective temperature, and the subsequent configurations remain local energy minima under AQS dynamics. For values of $\gamma_{max}$ close to $\gamma_{max}^Y$, the convergence to the steady state can be very slow and therefore, it is necessary to consider a large number of cycles [3] in such cases. The asymptotic, steady state, energies are obtained by stretched exponential fits of ($U/N$ *vs* $\gamma_{acc}$) as shown, and the final values are presented in

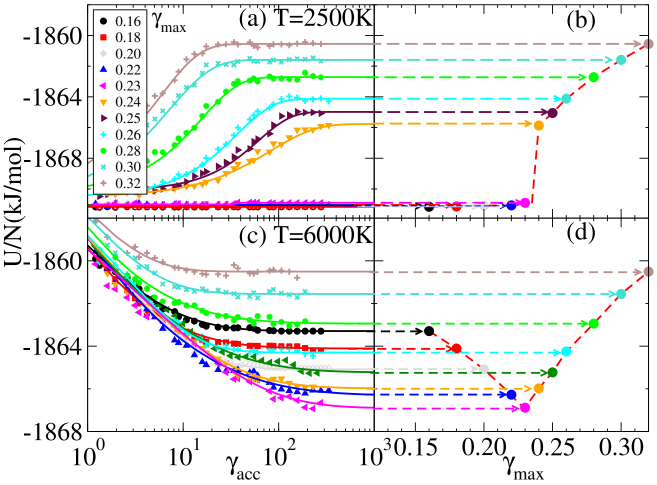


FIG. S1. Potential energy per atom $U/N$ against accumulated strain for zero-strain configurations, for (a) $T = 2500K$ and (c) $T = 6000K$ for several strain amplitudes $\gamma_{max}$, for number of atoms $N = 1728$. Data shown are averaged over 12 independent samples in each case. Solid lines through the data points are fits to a stretched exponential form. The asymptotic energies are plotted against $\gamma_{max}$ for (b) $T = 2500K$ and (d) $T = 6000K$.

Figs. S1(b) and S1(d) for different values of $\gamma_{max}$. The difference between the two cases is striking. For high $T$, the system anneals to lower energy states with increasing $\gamma_{max}$ until it yields at $\gamma_{max}^Y = 0.23$. For low $T$, the energy shows little evolution below yielding and a sudden jump when yielding occurs. Above yielding, the energies do not depend on the initial conditions, and attain the same $\gamma_{max}$ dependent values. The qualitative change in behavior illustrated occurs across a threshold temperature of $T_{th} = 3100K$ as discussed in detail in [4].

## S-3. ABSORBING TO DIFFUSIVE TRANSITION

The steady state can be characterized by inspecting atomic displacements and with this aim, we compute the sample (and initial configuration) averaged mean square displacement (MSD) between stroboscopic configurations (zero strain, separated by one or more cycles of shear) as a function of strain amplitude. The resulting curves are shown in Fig. S2(a) for $T = 2500K$ and in Fig. S2(b) for $T = 6000K$ and they present similar trends. For $\gamma_{max} < \gamma_{max}^Y$, the MSD does not change with accumu-

* sastry@jncasr.ac.in

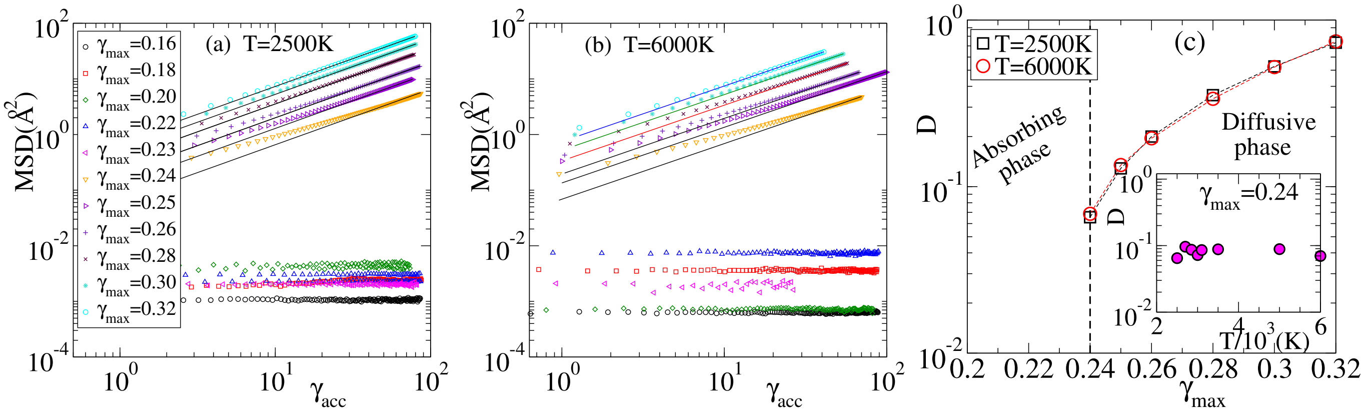

FIG. S2. Mean square displacement calculated in the steady state against accumulated strain difference $\gamma_{acc}$ for (a) $T = 2500K$ and (b) $T = 6000K$ for system size $N = 1728$. Data are averaged over ten samples. (c) Variation of the diffusion constant against strain amplitude for two different temperatures. Inset: $D$ against $T$ for given $\gamma_{max} = 0.24$, just above the yield strain amplitude.

lated strain difference $\gamma_{acc}$ and this indicates that the system has reached to an absorbing state where atoms come back to the same position after each cycle. On the other hand, for $\gamma_{max} > \gamma^{Y}_{max}$, the atomic motion is diffusive, as characterized by a linear dependence of MSD with accumulated strain difference beyond the initial transient period. Such diffusive motion can be characterized by an effective diffusion constant defined in terms of accumulative strain as,

$$MSD \sim D\gamma_{acc}. \tag{S2}$$

The extracted values of $D$ are presented in Fig. S2(e) as a function of strain amplitude for the two different temperatures. For both cases, we observe a finite jump at the critical strain amplitude implying a discontinuous yielding transition. The height of the jump, represented by the value of the diffusion coefficient just above the yield amplitude $\gamma^{Y}_{max}$, is found to be independent of the temperature of the parent liquid, as shown in inset of Fig. S2(c).

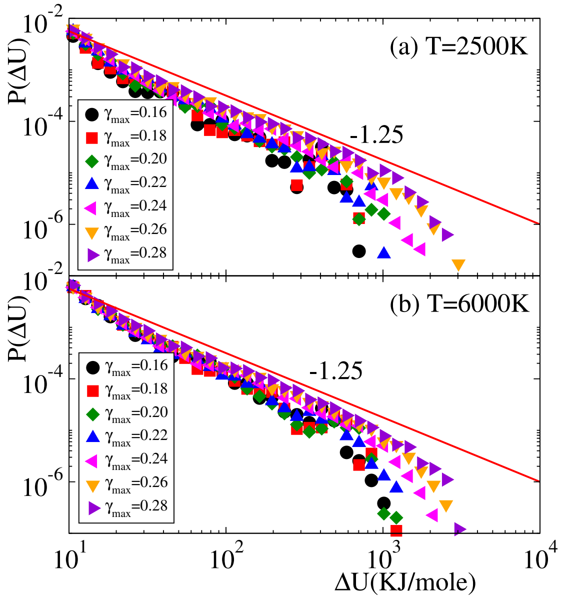

FIG. S3. Distributions of energy drops during an avalanche for (a) $T = 2500K$ and (b) $T = 6000K$ for a system with $N = 1728$ for several strain amplitudes. Solid lines are power laws with the exponent $-1.25$, shown for reference.

## S-4. ENERGY DROP STATISTICS

The plastic rearrangements of the system under cyclic deformation can be characterized by the statistics of energy drops during the minimization procedure in a deformation step. In Figs. S3 (a) and S3(b) the distributions of energy drops of the system in a plastic event are shown for two temperatures $T = 2500K$ and $6000K$, respectively. For both cases, we see a power law regime in the distribution, with a cut-off. The exponent of the power law is close to $-1.25$. The exponent value is the same as that observed in [5] for energy drops in the Kob-Andersen binary Lennard-Jones mixture, although in [5] the drops considered were for particles within a plastic rearrangement region. It is also apparent that the cut-off values, above which departure from the power law is observed, are larger for the distributions corresponding to $\gamma_{max} > \gamma^{Y}_{max}$, compared to those for $\gamma_{max} < \gamma^{Y}_{max}$.

## S-5. STATISTICS OF AVALANCHES

In this section, we present details of methods of analysis used to investigate avalanches, and additional supporting results, as follows:

- In Sec. S-5 A, we discuss in detail the use of local

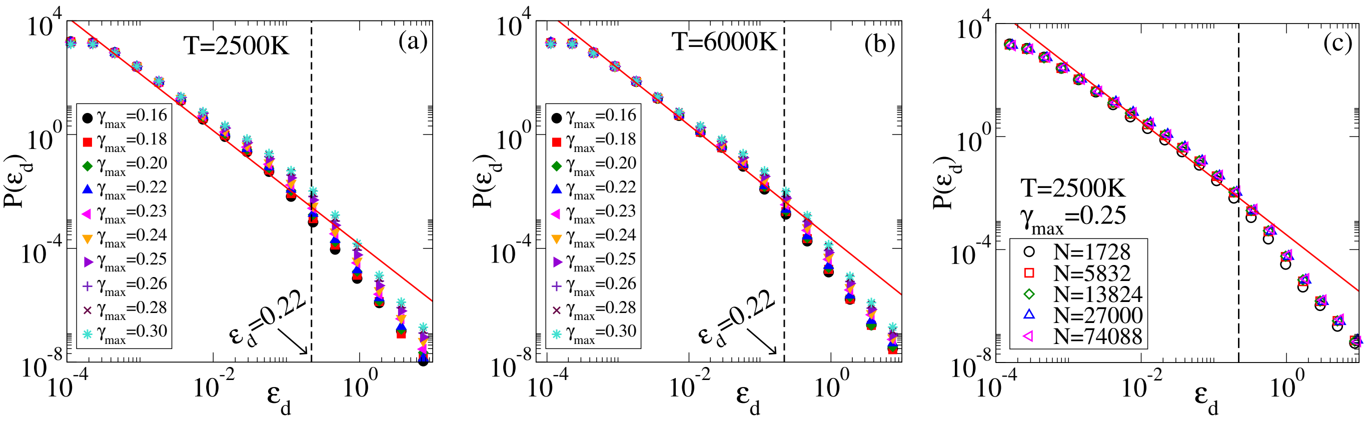


FIG. S4. Distributions of the local strain $\epsilon_d$ for different $\gamma_{max}$ for (a) $T = 2500K$ and (b) $T = 6000K$ for $N = 1728$. The expected [6] power-law with exponent $-2$ is shown by a red solid line. The vertical line represents the cutoff value of $\epsilon_d = 0.22$ beyond which the distributions deviate from the power law. (c) Plot of $P(\epsilon_d)$ against $\epsilon_d$ for different system sizes for $T = 2500K$ and strain amplitude $\gamma_{max} = 0.25$.

deviatoric stress to compute avalanche sizes (Fig. S4).

- In Sec. S-5 B, we present the avalanche statistics for $T = 6000K$, compare the mean cluster size results for $T = 2500K$ and $T = 6000K$, as well as the variation of the average cluster size with accumulated strain, in Fig S5. We provide a detailed description of the moment analysis to extract the exponent values corresponding to the distribution of avalanches, clusters, and the number of clusters. We describe additional supporting results for Fig. 1 of the main text, as well as for two additional values of $\gamma_{max}$ (Fig. S6, S8, S9). We also show data collapse of cluster size distributions for different choices of exponents in Fig. S7 to show that $\tau_c = 2$ is robustly obtained.

- In Sec. S-5 C, we explore different scaling relations between different exponents associated with avalanche size, cluster size and number of clusters. We show data for the mean number of clusters, mean cluster size as a function of avalanche size $S$ in Fig. S10, from which the exponents $\gamma_{ns}$ and $\tau$ are independently obtained.

- In Sec. S-5 D, we confirm that our present findings are consistent with the results for avalanches based on single particle displacements (Fig. S11), employed in [5].

- In Sec. S-5 E, we verify that the cluster size distribution employing deviatoric strain analysis reproduces the exponent for the cluster size distribution for the KA-BMLJ previously investigated in Ref. 5. (Fig. S12). We also show results for the distributions of avalanche size and the number of clusters in Fig. S13. In Fig. S14, we show the mean number of clusters and mean cluster size for avalanches of size $S$, and the conditional distribution of the number of clusters, for KA-BMLJ.

- In Sec. S-5 F, we compute the fractal dimension of largest clusters in an avalanche for silica and the KA-BMLJ (Fig. S15).

### A. Avalanche statistics employing the local deviatoric strain $\epsilon_d$

We compute the statistics of the size of clusters of active particles and avalanches during plastic rearrangements, considering the configurations before and after such events (stress drop) in the first quadrant of the strain cycle ($\gamma : 0 \to \gamma_{max}$). To identify the active particles, we employ the deviatoric local strain calculation as suggested by Salerno and Robbins in Ref. 6. To define the strain field, first the displacement of each atom is computed during an avalanche. The derivative of the displacement field is obtained through a finite difference method. A tetrahedral tiling is defined for the particle positions of the configuration before the avalanche. For each tetrahedron, we find the deformation gradient tensor $\mathbf{F}$ which maps each of the old nodal separation vectors, $\vec{r}_{ab}$, $\vec{r}_{ac}$, and $\vec{r}_{ad}$ into the new ones so that, $\vec{r}'_{ab} = \mathbf{F}\vec{r}^{ab}$, $\vec{r}'_{ac} = \mathbf{F}\vec{r}^{ac}$, $\vec{r}'_{ad} = \mathbf{F}\vec{r}^{ad}$. These three conditions give the 9 components of $\mathbf{F}$ uniquely for each tetrahedron. Knowing $\mathbf{F}$, the derivative of the displacement $\vec{u}$ along direction $i$ with respect to $x_j$ is obtained via $\frac{\partial u_i}{\partial x_j} = \mathbf{F_{ij}} - \delta_{ij}$. To eliminate the effect of any translations or rotations of the tetrahedron, the symmetrized strain tensor is then constructed as $\epsilon_{ij} = \frac{1}{2}\left(\frac{\partial u_i}{\partial x_j} + \frac{\partial u_j}{\partial x_i}\right)$. The deviatoric strain tensor is defined as $\epsilon_{\text{dev}} = \epsilon - d^{-1}\text{Tr}(\epsilon)\text{I}$ where $d = 3$ is the space dimension. The second deviatoric strain invariant $J_2 = \frac{1}{2}\text{Tr}(\epsilon^2_{\text{dev}})$ is used to obtain the shear strain,

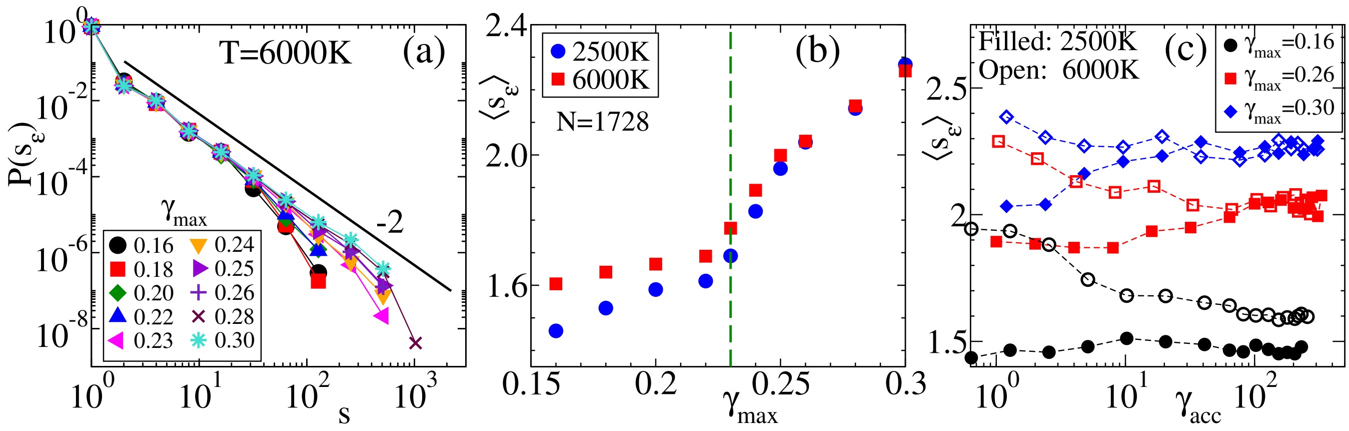


FIG. S5. (a) Cluster size distribution for $T = 6000K$ for several values of $\gamma_{max}$. (b) Variation of the average cluster size $\langle s_\epsilon \rangle$ in the steady state as a function of the strain amplitude $\gamma_{max}$ for $T = 2500K$ and $6000K$. (c) Evolution of the mean cluster size $\langle s_\epsilon \rangle$ with $\gamma_{acc}$ for different initial conditions ($T = 2500K$ and $6000K$) for three different strain amplitudes.

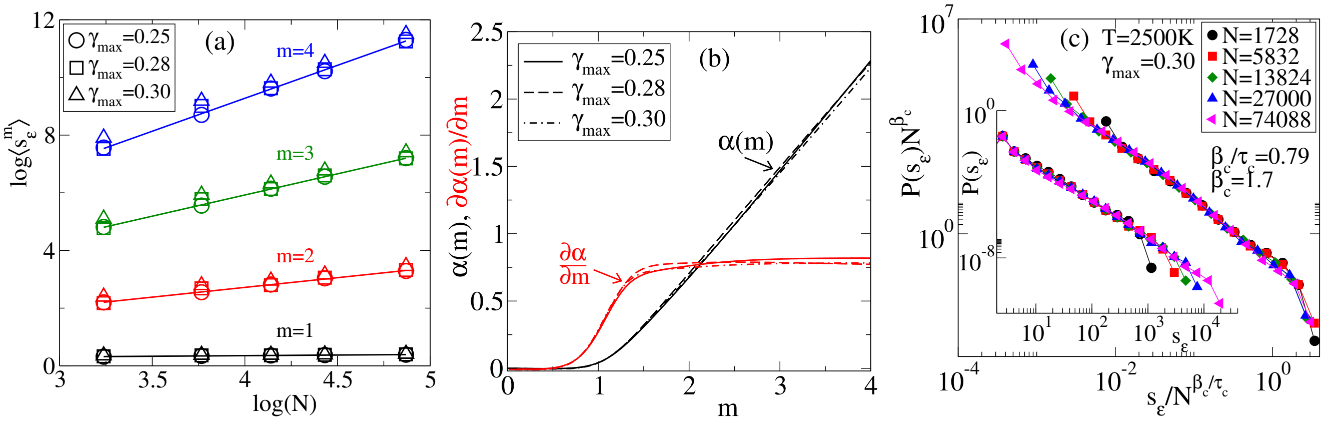


FIG. S6. **Moment analysis for cluster size $s_\epsilon$ and data collapse:** (a) various moments of the cluster size distribution $\langle s_\epsilon^m \rangle$ against system size for three different strain amplitudes $\gamma_{max} = 0.25, 0.28$ and $0.30$. (b) The moment exponent $\alpha(m)$ (black lines) and its derivative $\partial\alpha(m)/\partial m$ (red lines) against $m$ for $\gamma_{max} = 0.25$ (solid line), 0.28 (dashed line) and 0.30 (dotted dashed line). Note that the error in $\alpha(m)$, which is measured by least square fitting through the data points, increases with $m$, attaining a maximum of 2% at $m = 4$. (c) The scaled distribution $P(s_\epsilon)N^{\beta_c}$ against scaled variable $s_\epsilon/N^{\beta_c/\tau_c}$ for different system size $N$ for $\gamma_{max} = 0.30$. The unscaled data are shown in the inset.

defined as $\epsilon_d = \sqrt{J_2}$. In response to a local perturbation, the elastic strain varies as $\epsilon \sim r^{-d}$ where $r$ is the distance from the location of perturbation [7–10]. The distribution of $\epsilon_d$ arising from such elastic response follows a power law, $P(\epsilon_d) \sim \epsilon_d^{-2}$, obtained from considering $r^{d-1}dr \sim P(\epsilon_d)d\epsilon_d$. The deviation from such power law behavior is employed to identify a threshold for $\epsilon_d$ beyond which the strains can be identified as having arisen from plastic rearrangements [6].

In Fig. S4(a) and S4(b), we present the distributions of $\epsilon_d$, $P(\epsilon_d)$, for $T = 2500K$ and $6000K$ respectively for $N = 1728$ for several strain amplitudes. In Fig. S4(c) we present $P(\epsilon_d)$ for different system sizes for a given strain amplitude. As expected, the distributions follow the elastic power-law behaviour up to a value $\epsilon_d = 0.22$ beyond which the distribution deviates from the power law. This threshold allows us to identify the active particles belonging to regions of plastic rearrangement. In analysing cluster statistics, two active particles are considered to belong to the same cluster if they are separated by a distance $< 2.05\mathring{A}$, the first co-ordination shell of the silica.

### B. Moment analysis and finite size scaling

As discussed in the main text, the exponent $\tau_c$ of the cluster size distribution is found to be $\sim 2$ above yielding. This result is different from that of the 3D KA-BMLJ model where the 3/2 has been observed [5]. In order to characterize the statistics size better, we perform a finite size analysis by simulating several system sizes, $N = 1728, 5832, 13824, 27000, 74088$ for three different strain amplitudes $\gamma_{max} = 0.25, 0.28$ and $0.30$ above

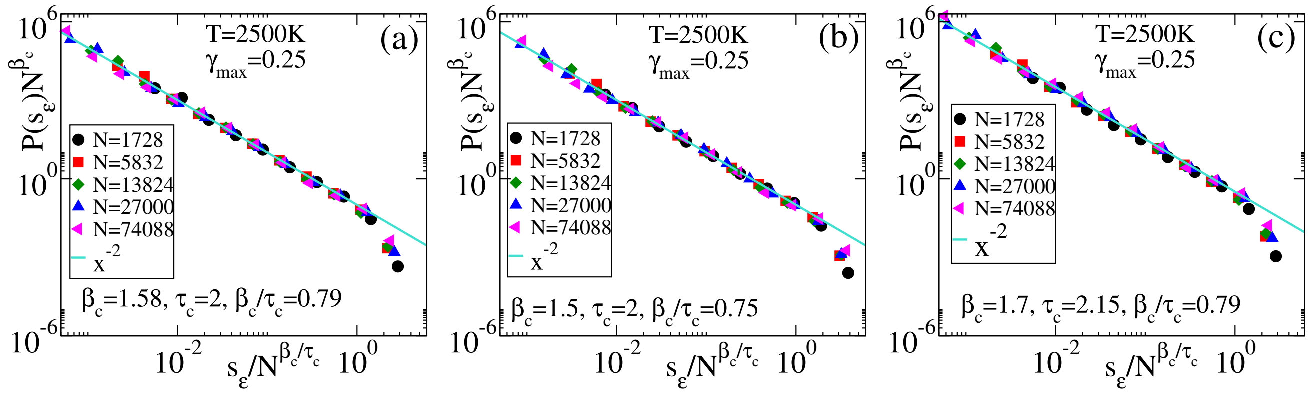


FIG. S7. **Data collapse for the cluster size distribution:** Scaled distribution $P(s_\epsilon)N^{\beta_c}$ against scaled variable $s_\epsilon/N^{\beta_c/\tau_c}$ for different system size $N$ for $\gamma_{max} = 0.25$ using different values of exponents $\beta_c$ and $\tau_c$. Blue solid line indicates the power-law with exponent $-2$ in all the cases.

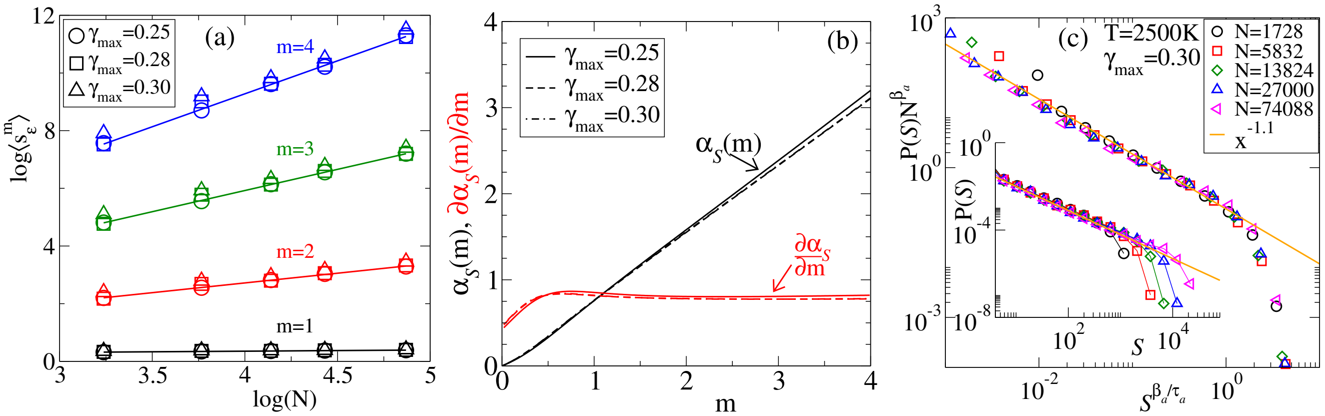


FIG. S8. **Moment analysis for avalanche size $S$ and data collapse:** (a) Various moments of the avalanche size distribution $\langle S^m \rangle$ against system size for $\gamma_{max} = 0.25, 0.28$ and $0.30$. (b) Moment exponent $\alpha_S(m)$ (black lines) and its derivative $\partial\alpha_S(m)/\partial m$ (red lines) against $m$ for $\gamma_{max} = 0.25$ (solid line) 0.28 (dashed line) and 0.30 (dotted dashed line). (c) The scaled distribution $P(S)N^{\beta_a}$ against scaled variable $S/N^{\beta_a/\tau_a}$ for different system size $N$ for $\gamma_{max} = 0.30$. The unscaled data are shown in the inset.

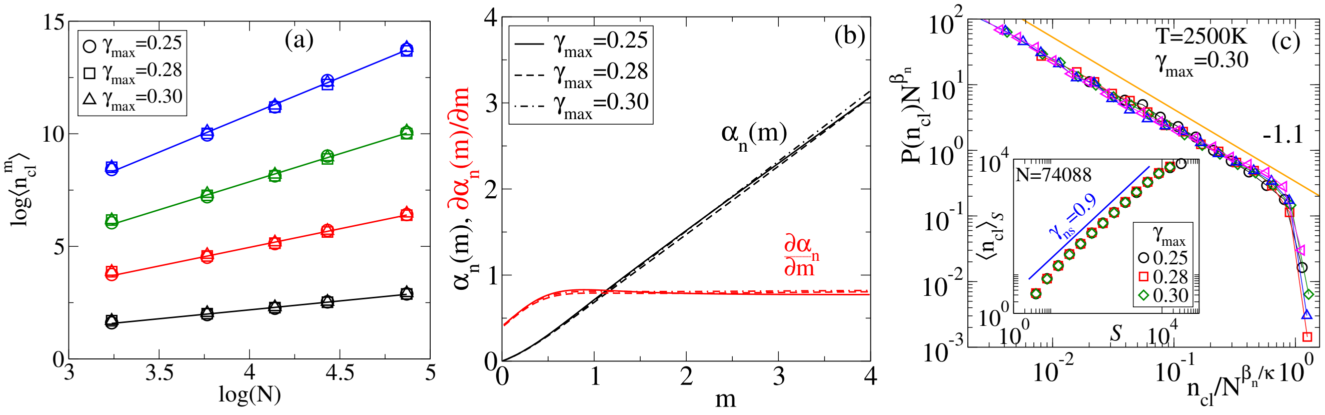


FIG. S9. **Moment analysis for number of clusters $n_{cl}$ and data collapse:** (a) Various moments of the cluster number distribution $\langle S^m \rangle$ against $N$ different $\gamma_{max}$. (b) Moment exponent $\alpha_n(m)$ (black lines) and its derivative $\partial\alpha_n(m)/\partial m$ (red lines) (c) The scaled distribution $P(n_{cl})N^{\beta_n}$ for different system size $N$ to obtain data collapse for $\gamma_{max} = 0.30$. Inset shows the variation $\langle n_{cl} \rangle \sim S^{\gamma_{ns}}$ with $\gamma_{ns} \approx 0.9$ .

the yield strain amplitude $\gamma^Y_{max} = 0.23$. We begin by analyzing the cluster size ($s$) distribution and subsequently

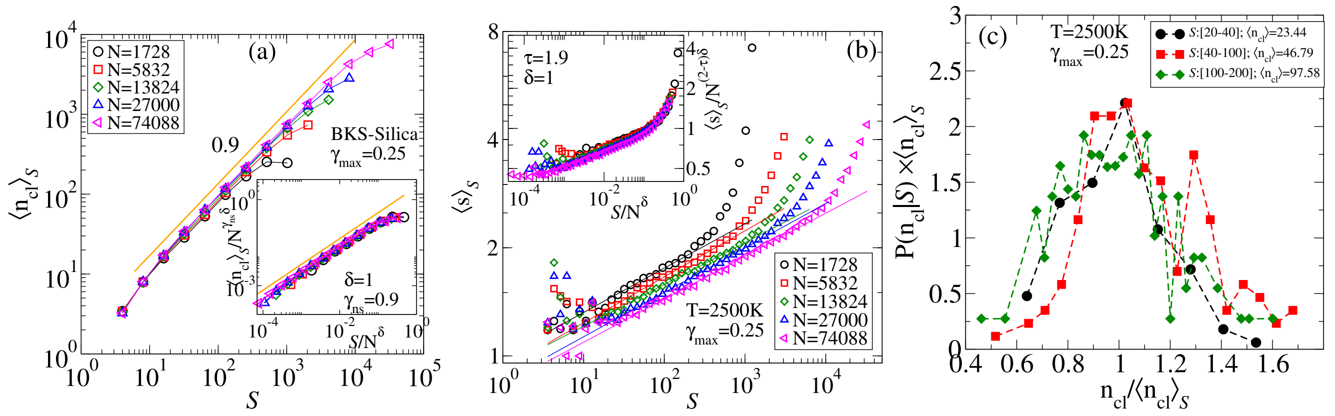


FIG. S10. (a) Average number of clusters for given avalanche size $S$ for different system sizes with $\gamma_{max} = 0.25$. Inset shows the data collapse. (b) Average cluster size for a given $S$ for different $N$ shows the scaling behaviour $\langle s\rangle_S \sim S^{2-\tau}$ with $\tau = 1.9$. Inset shows the data collapsed data with $\delta = 1$. (c) Scaled conditional probability distribution of the number of clusters for given avalanche size $S$ for a system of size $N = 74088$. Legends indicate the range of $S$ values and the mean number of clusters.

we perform the same analysis for the avalanche size ($S$) and number of clusters ($n_{cl}$). For finite size analysis, the scaling form of the cluster size distribution is assumed to be

$$P(s_\epsilon) \approx N^{-\beta_c} f\left[\frac{s_\epsilon}{N^{\beta_c/\tau_c}}\right] \tag{S3}$$

where the scaling function $f(x) \to x^{-\tau_c}$ for $x \to 0$, so that the power-law behaviour $P(s_\epsilon) \sim s_\epsilon^{-\tau_c}$ is recovered for small $s_\epsilon$ and $f(x)$ decreases to zero sufficiently fast when $x \to 1$. To extract the value of $\beta_c$ and $\tau_c$ we obtain the moments of the distribution function [11, 12] defined as:

$$\langle s_\epsilon^m\rangle = \int_0^\infty s_\epsilon^m P(s_\epsilon) ds = \int_0^\infty s_\epsilon^m N^{-\beta_c} f(s_\epsilon/N^{\beta_c/\tau_c}) ds_\epsilon$$
$$= N^{(\beta_c/\tau_c)(m+1-\tau_c)} \int_0^\infty z^m f(z) dz \tag{S4}$$

where, in the last step we introduce the variable $z = s_\epsilon/N^{\beta_c/\tau_c}$. Since the last integral is a constant, the moment $\langle s_\epsilon^m\rangle$ should vary with system size as

$$\langle s_\epsilon^m\rangle \sim N^{\frac{\beta_c}{\tau_c}(m+1-\tau_c)} \sim N^{\alpha(m)}, \tag{S5}$$

where

$$\alpha(m) = \frac{\beta_c}{\tau_c}(m + 1 - \tau_c) \tag{S6}$$

is the moment exponent.

Before discussing higher moments, we will present the data for first moment of the distribution function that represents the mean cluster size. Before that, in Fig. S5(a), we present the distribution of cluster sizes for $T = 6000K$, $N = 1728$, that complements the results shown in Fig. 1 or the main text. In Fig. S5(b), we show the variation of the first moment with $\gamma_{max}$. It is clear that, beyond $\gamma^Y_{max} = 0.23$, $\langle s_\epsilon\rangle$ increases rapidly due to the appearance of system-spanning avalanches. In Fig. S5(c), the evolution of $\langle s_\epsilon\rangle$ is presented as a function of $\gamma_{acc}$ for three representative values of $\gamma_{max}$ for $T = 2500K$ and $6000K$. It is interesting to observe that although $\langle s_\epsilon\rangle$ for different initial glasses evolves differently, their steady state properties are more or less same for a given strain amplitude, if $\gamma_{max} > \gamma^Y_{max}$.

In the Fig. S6, we present the same analysis as in Fig. 1 of the main paper for three different values of $\gamma_{max}$, for $T = 2500K$. Fig. S6 (a) shows the data of $\log\langle s_\epsilon^m\rangle$ against $\log N$ for $m = 1, 2, 3$, and 4 for different values of the strain amplitude. We calculate the moment exponent $\alpha(m)$ for values of $m$ ranging from 0.01 to 4 with an increment of 0.01. The derivative $\alpha' = \partial\alpha(m)/\partial m$ is computed numerically with the central difference method. In Fig S6 (b) we present the variation of $\alpha(m)$ and $\alpha'(m)$ with $m$. It can be seen that for all $\gamma_{max}$, $\alpha'$ saturates satisfactorily for $m > 2$.

We extract the values of exponents $\beta_c/\tau_c$ and $\tau_c$ using Eq. (S6) in two different ways. First, for each $\gamma_{max}$, we obtain the $\beta_c/\tau_c$ value from the saturated value of $\alpha'(m)$ at $m = 4$ and note the corresponding value of $\alpha(m = 4)$. We then solve Eq. (S6) to compute $\tau_c$. In a second method, we consider the values of $\alpha(m)$ for a wide range of $m$. For each $\gamma_{max}$, we fit the moment scaling exponent over the range $m = 3$ to $m = 4$ with a linear form to obtain the slope (which is equal to $\beta_c/\tau_c$) and intercept (which is $(\beta_c/\tau_c - \beta_c)$) and from these we calculate the $\tau_c$ value. From both the methods we find similar values of $\tau_c$, and we compute the average of the two. Finally the averaged values of $\tau_c = 2.15 \pm 0.07$ and $\beta_c/\tau_c = 0.79 \pm 0.02$ are obtained by considering the estimates for the three $\gamma_{max}$ values we consider. Error bar represents the maximum deviation of the data from the average value.

The estimate $\tau_c = 2.15 \pm 0.07$ is slightly larger than the value $\tau_c = 2$ in the data shown in Fig. 1 of the main text. Moreover, when we use the values $\tau_c = 2.15$ and

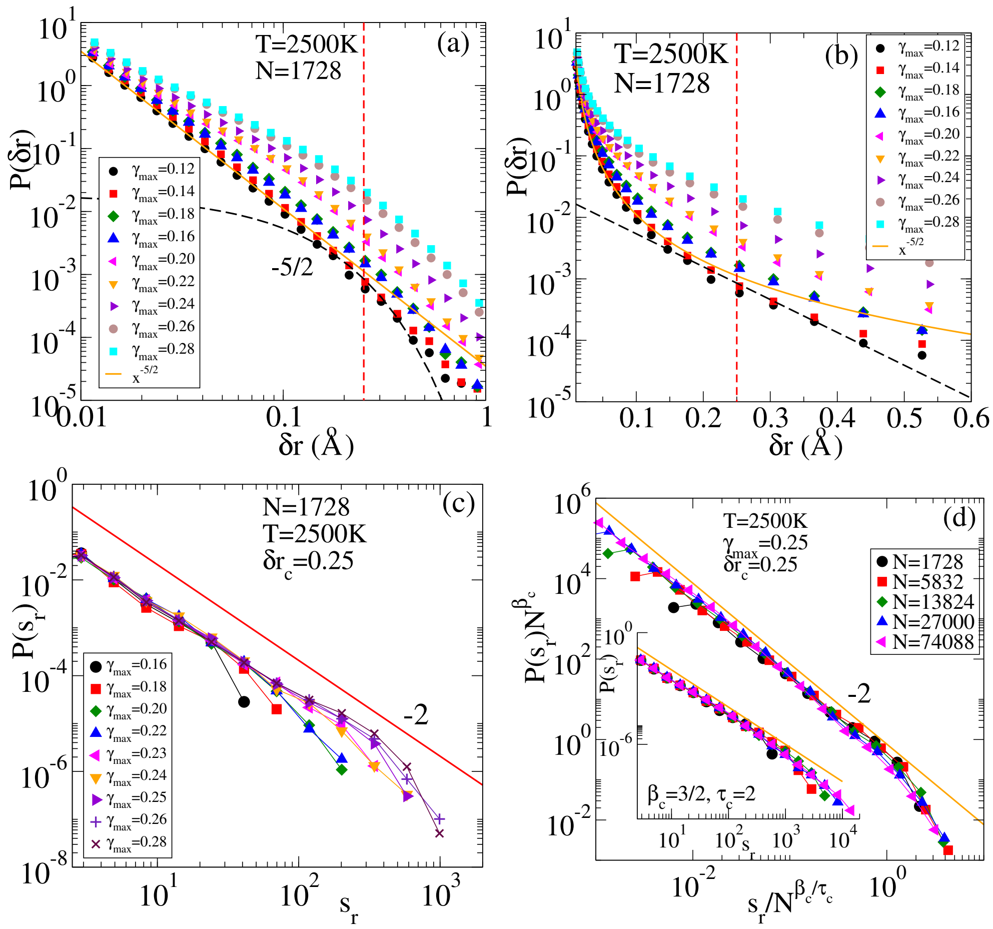


FIG. S11. Distributions of the particle displacements $\delta r$ during plastic events shown in (a) log-log and (b) semi-log scales for several strain amplitudes. For small displacements $\delta r$ the distribution follows a power-law with exponent $-5/2$ with an exponential tail represented by the orange solid line and the black dashed line respectively. The vertical line indicates the cutoff value of $\delta r = 0.25$ for the crossover from the power-law to exponential behavior. (c) $P(s_r)$, the distribution of the size of clusters ($s_r$) of active particles for different strain amplitude (and fixed system size $N$). (d) For a fixed strain amplitude, scaled cluster size distributions are shown for different system sizes. The power-law with the expected exponent of $-2$ is indicated by the solid line. Inset of (d) shows the corresponding unscaled distributions.

$\beta_c/\tau_c = 0.79$ to perform a scaling collapse of the distributions, shown in Fig. S7 (c), for $T = 2500K$, $\gamma_{max} = 0.25$, while the scaling collapse is very satisfactory, the resulting collapsed data are very well described by an exponent $\tau_c = 2$, rather than $\tau_c = 2.15$. To interrogate this further, in S7 (a),(b), we show the scaling collapse for two other choices of exponents, namely $\beta_c/\tau_c = 0.79$, $\tau_c = 2$ in (a) and $\beta_c/\tau_c = 0.75$, $\tau_c = 2$ in (b). The scaling collapse in these cases is equally satisfactory, and once again, the collapsed data are very well described by the exponent $\tau_c = 2$. Thus, within the small errors inherent in our analysis, we conclude that the cluster size distributions are robustly described by $\tau_c = 2$.

Similarly to the analysis above, we assume the finite size scaling form of the distribution of avalanche sizes $S$ and number of clusters $n_{cl}$ as

$$P(S) \approx N^{-\beta_a} f_a \left[ \frac{S}{N^{\beta_a/\tau_a}} \right] \quad \text{(S7)}$$

and

$$P(n_{cl}) \approx N^{-\beta_n} f_n \left[ \frac{n_{cl}}{N^{\beta_n/\kappa}} \right] \quad \text{(S8)}$$

where we use the subscript $a$ and $n$ for avalanche size and cluster number respectively. As described before we evaluate various moments and the associated moment exponents as shown in Figs. S8 and S8. Following a similar procedure as mentioned for $s_\epsilon$, we evaluate the values of exponents as $\beta_a/\tau_a = 0.79 \pm 0.02$, $\tau_a = 1.1 \pm 0.05$ for avalanche size, whereas, for the cluster number we find $\beta_n/\kappa = 0.78 \pm 0.03$ and $\kappa = 1.12 \pm 0.08$. Using these values we have a very reasonable data collapse for different system sizes as shown in Figs. S8(c) and Figs. S9(c), for $S$ and $n_{cl}$ respectively. Unlike the case of cluster size, the collapsed data for $S$ and $n_{cl}$ are well described by the exponents $\tau_a$ and $\kappa$ we determine by the moment analysis.

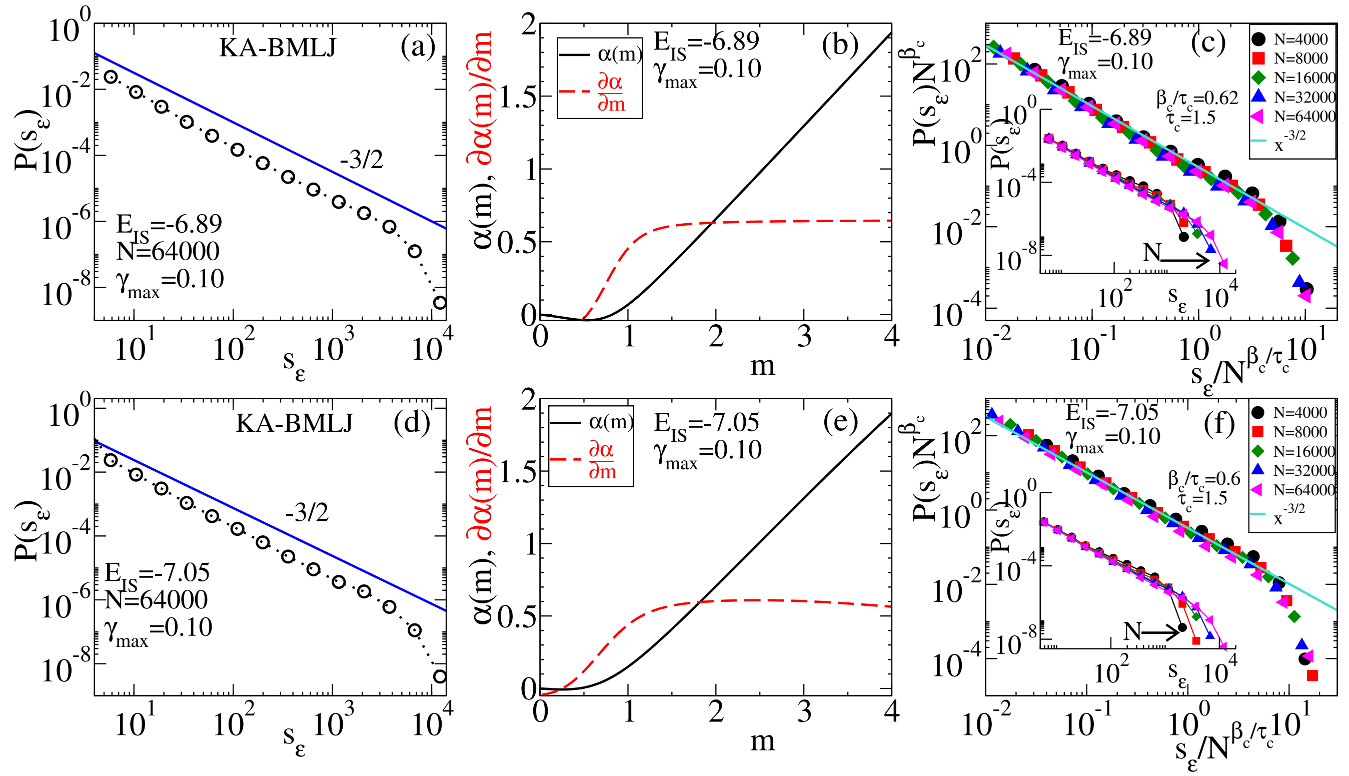


FIG. S12. Cluster statistics for the KA-BMLJ model: Distribution of the size of clusters of active particles identified from the local deviatoric strain analysis for (a) poorly annealed (initial inherent structure energy $E_{IS} = -6.89$) and (d) well annealed ($E_{IS} = -7.05$) glasses for $N = 64000$ using the cutoff $\epsilon_d = 0.20$. Variation of the moment exponent $\alpha(m)$ and its derivative $\partial\alpha(m)/\partial m$ for (b) the poorly annealed glass and (e) well annealed glass. The scaled cluster size distribution $P(s_\epsilon)N^{\beta_c}$ against scaled variable $s_\epsilon/N^{\beta_c/\tau_c}$ with $\beta_c/\tau_c = 0.6$ and $\tau_c = 3/2$ for different system sizes to obtain the data collapse for (c) $E_{IS} = -6.89$ and (f) $E_{IS} = -7.05$; insets show the unscaled data.

### C. Exponent relations

Next we obtain a relation among $\tau_a$, $\tau_c$ and $\kappa$, following an analysis related to that in [13], but as we see below, our analysis leads to a new relationship between exponents $\tau_a$, $\tau_c$ and the exponent $\tau$ that describes the conditional distribution of cluster sizes.

With the definition of the avalanche size $S$,

$$S = \sum_{i=0}^{n_{cl}} s_i, \tag{S9}$$

we consider the number of clusters of a given size $n(s|S)$ in an avalanche of size $S$. By definition, we have

$$\int_1^S s\ n(s|S)\ ds = S. \tag{S10}$$

Likewise, by definition, the total number of clusters present is given by

$$\int_1^S n(s|S)\ ds = n_{cl}(S). \tag{S11}$$

As discussed in [13], $n(s|S)$ is broadly distributed, and we thus assume $n(s|S) = As^{\tau}$, and the condition Eq. S10 requires $A = (2-\tau)S^{\tau-1}$ (for large $S$). Importantly, we allow $\tau \neq \tau_c$ in our analysis. Assuming $\tau > 1$, we obtain, straight forwardly,

$$n_{cl}(S) \sim S^{\tau-1} \sim S^{\gamma_{ns}} \tag{S12}$$

which defines the exponent $\gamma_{ns}$. The above form for $n(s|S)$ also means that the mean cluster size is given by

$$\langle s\rangle_S \sim S^{2-\tau}. \tag{S13}$$

Eq. S12 leads to the exponent relation

$$\gamma_{ns} = \tau - 1. \tag{S14}$$

The above relation can also by obtained by noting that $\langle s\rangle_S = S/\langle n_{cl}\rangle_S$ as done in [13].

We show the variation of $\langle n_{cl}\rangle_S$ with $S$ in the inset of Fig. S9 (c) where we find $\gamma_{ns} \approx 0.9$ which is not consistent with the $\tau_c$ value we discussed earlier. To investigate this further, we shown in Fig. S10 (a) $\langle n_{cl}\rangle_S$ for a range of system sizes. We also show a corresponding data col-

lapse, with scaling exponents $\gamma_{ns}$ and $\delta$ (the significance of the exponent $\delta$ needs further investigation and we do not discuss further). The estimated exponent is clearly $\gamma_{ns} = 0.9$. In S10 (c), we show the conditional distribution $P(n_{cl}|S)$. The data are noisy, but they show the same form with a peaked distribution as seen in [13]. In S10 (b) we show the corresponding data for the mean cluster size, $\langle s \rangle_S$ which are well described by $\tau = 1.9$. Note that $\langle s \rangle_S$ should have no $S$ dependence if the relevant exponent is $\tau_c = 2$.

Since the number of clusters $n_{cl}$ for a given avalanche size $S$ are distributed around a mean $\langle n_{cl} \rangle_S$, we assume the conditional probability $P(n_{cl}|S) \approx S^{-\gamma_{ns}} g(n_{cl}/\langle n_{cl} \rangle_S)$, so that Eq. (S12) can be obtained using $\langle n_{cl} \rangle_S = \int n_{cl} P(n_{cl}|S) dn_{cl}$. Likewise, the total distribution can be expressed in terms of $P(n_{cl}|S)$ as

$$P(n_{cl}) = \int P(n_{cl}|S)P(S)ds \sim n_{cl}^{1+(\tau_a-1)/\gamma_{ns}}. \tag{S15}$$

Altogether, using $P(n_{cl}) \sim n_{cl}^{-\kappa}$ and Eqs. (S14), and (S15) we find the scaling relation

$$\kappa = 1 + \frac{\tau_a - 1}{\tau - 1}. \tag{S16}$$

This identity is well satisfied with the measured values of the exponents $\tau = 1.9$, $\tau_a = 1.1$ and $\kappa = 1.12$ as obtained from finite size analysis.

Finally, we consider the relation between exponents $\tau$, $\tau_a$ and $\tau_c$. We consider the normalised $n(s|S)$ describe above, to obtain the distribution $P(s|S) \sim s^{-\tau}$. We further assume the distribution of avalanches to be given by $P(S) \sim S^{-\tau_a}$. From these, the full distribution of $s$ can be written as

$$P(s) = \int_s^\infty P(s|S)P(S)dS \sim s^{-(\tau+(\tau_a-1))}. \tag{S17}$$

Thus, the exponent describing the cluster sizes is

$$\tau_c = \tau + (\tau_a - 1). \tag{S18}$$

The values of $\tau = 1.9$ and $\tau_a = 1.1$ lead to $\tau_c = 2$, which is indeed the value obtained from the analysis above. To our knowledge, this relationship has not previously been discussed.

### D. Avalanche statistics based on single particle displacements $\delta r$

The active particles during plastic rearrangements can also be identified using the method based on single particle displacements $\delta r$ [5, 14]. We confirm, in this section, that this method leads to results that are consistent with those obtained using the local deviatoric strain analysis. During a plastic rearrangement, it is found that the distribution of single particle displacements $P(\delta r)$ displays a power law distribution at small values with an exponent of $-5/2$ and an exponential tail that corresponds to plastic displacements. The power-law exponent $-5/2$ can be deduced from linear elasticity assuming that the system outside the plastic core undergoes an elastic deformation due to the stresses created by the plastic rearrangement, and is thus equivalent to the discussion in relation to the deviatoric strain approach above. In Figs. S11 (a) and S11 (b) we present the data of $P(\delta r)$ in log-log and log-linear representation respectively. Clearly, for small amplitudes the distributions exhibit a power-law form, with an exponential tail at large value of $\delta r$. Noticeably, the location of the crossover from power-law to exponential form depends on the strain amplitude and above yielding the distinction between the two regimes is not very clear. However, even with these limitations, one can choose the smallest cutoff of $\delta r$ as $0.25\mathring{A}$ based on the data for the lowest amplitude $\gamma_{max} = 0.12$ so that the active particles in a plastic rearrangement at all $\gamma_{max}$ can be detected. We label the particles as active if they are displaced by more than $0.25\mathring{A}$. To analyze the cluster statistics, two active particles are considered to belong to the same cluster if they are separated by a distance $< 2.05\mathring{A}$, or, be within the first co-ordination shell of the silicon atoms. We refer to the cluster sizes obtained as $s_r$ to distinguish from the cluster sizes $s_\epsilon$ obtained using the deviotoric strain definition. The cluster size distributions obtained by this method are presented in Fig. S11 (c) for different strain amplitudes for a given system size, and in Fig. S11 (d) for different system sizes for a given strain amplitude. The resulting distributions confirm that the power-law exponent is $\sim 2$. The inset of Fig. S11 (d) represents the data collapse of distributions for different system sizes with the same values of exponents obtained through deviatoric strain method. We conclude that the deviatoric and the displacement field methods are indeed consistent.

### E. Avalanche analysis for 3D KA-BMLJ

So far, it has been seen that for BKS Silica both the deviatoric strain and the displacement field methods of identifying active particles lead to distributions of cluster sizes with exponent $\tau_c = 2$. However, for the 3D Kob-Andersen binary mixture Lennard-Jones(KA-BMLJ) model the cluster size distribution has been shown to exhibit a power-law scaling with $\tau = 3/2$, the mean field value using a displacement field analysis [5]. To verify consistency, we analyse the cluster size statistics of the KA-BMLJ model with the local deviatoric strain method. The $\epsilon_d$ are computed as described before and their distribution displays the expected power-law ($P(\epsilon_d) \sim \epsilon_d^{-2}$) with deviations at large values of $\epsilon_d$. We choose the cutoff value as $\epsilon_d = 0.20$ for the identification of active particles. The cluster sizes of active particles are computed considering two particles to be in the

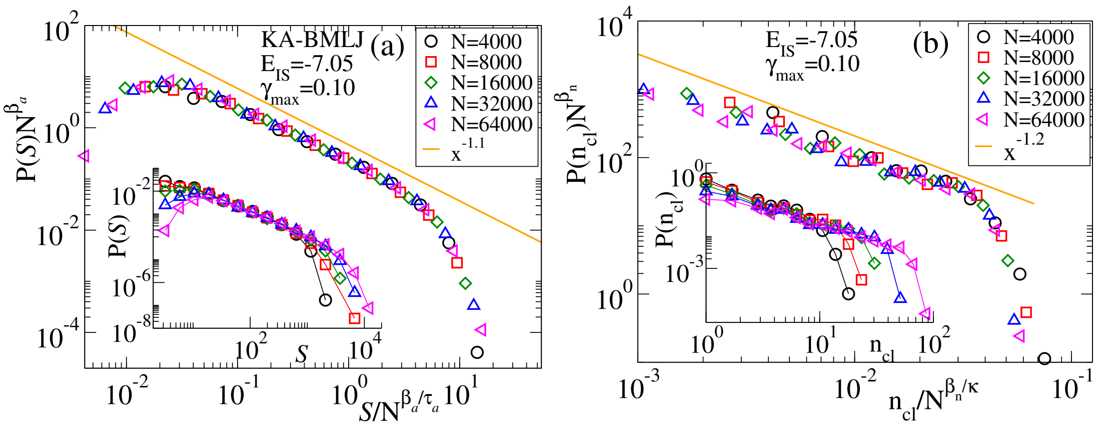


FIG. S13. (a) Scaled avalanche size distribution and (b) Scaled distribution of the number of clusters for different system sizes for well annealed $E_{IS} = -7.05$ KA-BMLJ. Data collapse is obtained using $\beta_a/\tau_a = 0.66$, $\tau_a = 1.1$ for avalanche size and $\beta_n/\kappa = 0.6$, $\kappa = 1.2$. Insets show the unscaled data.

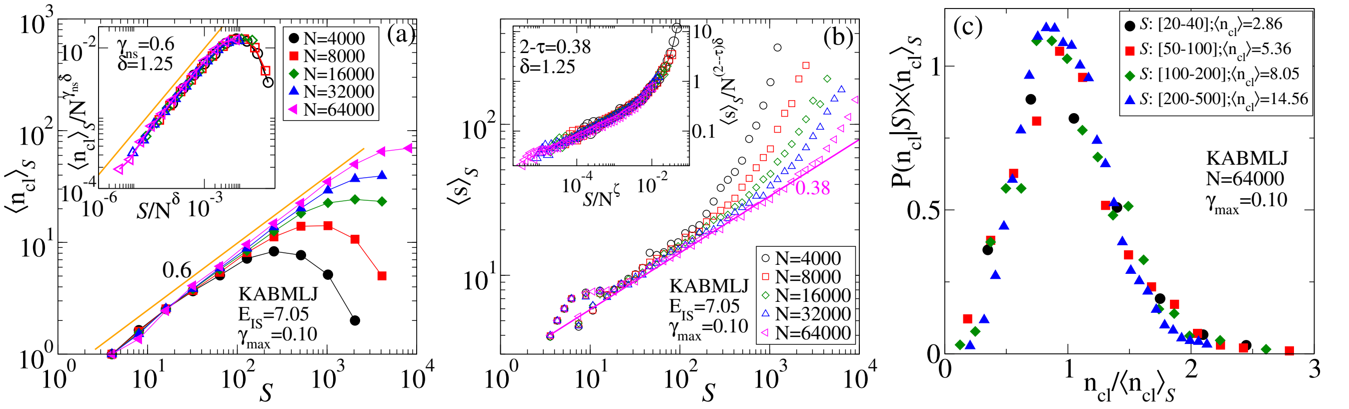


FIG. S14. **Conditional quantities of KA-BMLJ:** (a) Average number of clusters for given avalanche size $S$ for different system sizes for $\gamma_{max} = 0.10$. Inset shows the data collapse using $\gamma_{ns} = 0.6$ and $\delta = 1.25$. (b) Average cluster size for a given $S$ for different $N$ shows $\langle s\rangle_S \sim S^{0.38}$ scaling behaviour. Inset shows the collapsed data with $\delta = 1.25$. (c) Scaled conditional probability distribution of the number of clusters for given avalanche size $S$ for a system of size $N = 74088$. Legends indicate the range of $S$ values and the mean number of clusters.

same cluster if they are less than the distance $1.4\sigma_{AA}$ apart, corresponding to the first co-ordination shell for this model. In Figs. S12 (a) and (d) we present the distribution of cluster sizes for two different KA-BMLJ glasses (poorly annealed and well annealed) for $N = 64000$. For both cases, we observe the power-law behaviour with exponent $\tau_c = 3/2$ with a cutoff. We perform the moment analysis considering different system sizes. In Figs. S12 (b) and (e) we show the moment exponent and its derivative. We observe that the derivative converges to $\beta_c/\tau_c \approx 0.6$. We also see that for the poorly annealed case $\partial\alpha(m)/\partial m$ does not converge within the $m < 4$ range, and the ratio of second to the first moment scales $N^{0.36}$ in agreement what was observed in Ref. 5. However the ratio of two consecutive moments in large limit of $m$ scales as $N^{0.6}$ for both the glasses. With $\tau_c = 3/2$ and $\beta_c/\tau_c = 0.6$ we perform the data collapse as presented in Figs. S12 (c) and (f) for both the glasses. This analysis confirms the finding in [5] and validates the analysis performed in the present manuscript. Additionally we also study the avalanche size and cluster number statistics for KA-BMLJ model. In Figs. S13(a) and S13 (b) we show the finite size data collapse which reveals $\beta_a/\tau_a = 0.66$, $\tau_a = 1.1$ for avalanche size and $\beta_n/\kappa = 0.6$ and $\kappa = 1.2$. Interestingly, we find the same power-law exponent $\tau_a = 1.1$ associated with the avalanche size distribution for both Silica and KA-BMLJ, though the cluster number and cluster size exponents are different.

In Fig. S14 we show various conditional quantities and related data collapse. Fig. S14(a) shows the variation of mean number of clusters for a given avalanche size $S$ that clearly demonstrates $\gamma_{ns} = 0.6$. As shown in Fig. S14(b) average cluster size for fixed avalanche size grows as $\langle s\rangle_S \sim S^{2-\tau} \sim S^{1-\gamma_{ns}}$, with $\tau$ estimated to be $\tau = 1.62$. These values of the exponents is again consistent with the scaling relation Eq. (S14). The expression for $\kappa$, Eq. S16 is also reasonably well satisfied. However, the relation in Eq. S18 is not satisfied, and these discrep-

| | Shear protocol | System | Scaling form | Exponent $\tau$ | $\alpha$ | Ref. |
|---|---|---|---|---|---|---|
| Molecular dynamics simulation | Uniform shear | LJ 2D | $P(\delta E) \sim \delta E^{-\tau} f(\delta E/L^{\alpha})$ | 1.25 | 1.6 | [6] |
| | | LJ 3D | $P(\delta E) \sim \delta E^{-\tau} f(\delta E/L^{\alpha})$ | 1.2 | 2.1 | [6] |
| | | LJ 2D | $P(\delta\sigma) \sim \delta\sigma^{-\tau} f(\delta\sigma/L^{\alpha})$ | 1.28 | 0.9 | [15] |
| | | LJ 3D | $P(\delta\sigma) \sim \delta\sigma^{-\tau} f(\delta\sigma/L^{\alpha})$ | 1.25 | 1.3 | [15] |
| | | LJ 2D | $P(\delta\sigma) \sim \delta\sigma^{-\tau} f(\delta\sigma/L^{\alpha})$ | 1.1 | 1.23 | [16] |
| | | LJ 2D | $P(\delta\sigma) \sim \delta\sigma^{-\tau} f(\delta\sigma/L^{\alpha})$ | 1.493 | 1.034 | [17] |
| | | LJ 3D | $P(s) \sim s^{-\tau}$ | 2.39 | | [18] |
| | | Cu-Zr 3D | $P(\delta\sigma) \sim \delta\sigma^{-\tau}$ | 1.5 | | [19] |
| | | POLY 3D | $P(\delta\sigma) \sim \delta\sigma^{-\tau} f(\delta\sigma/L^{\alpha})$ | 1.25 | 1.5 | [20] |
| | | SW-Si 3D | $P(S) \sim S{-}\tau$ | 1.96 | | [21] |
| | Tensile deformation | CU-Zr 3D | $P(\delta\sigma) \sim \delta\sigma^{-\tau}$ | 1.25 | | [22] |
| | Cyclic shear | LJ+hump 2D | $P(\delta E) \sim \delta E^{-\tau} f(s(\gamma^{Y}_{max} - \gamma_{max})^{\delta})$ | 1.04 | $\delta = 2.1$ | [23] |
| | | LJ 3D | $P(s) \sim s^{-\tau}$ | 1.5 | | [5] |
| Elastoplastic model | Uniform shear | 2D | $P(\delta E) \sim \delta E^{-\tau} f(\delta E/L^{\alpha})$ | 1.28 | 0.9 | [15] |
| | | 2D | $P(\delta\sigma) \sim \delta\sigma^{-\tau}$ | 1.25 | | [24] |
| | | 2D | $P(\delta s) \sim \delta s^{-\tau} f(\delta s/L^{\alpha})$ | 1.36 | 1.1 | [25, 26] |
| | | 2D & 3D | $P(S_t) \sim \delta S_t^{-\tau}$ | $1.25 - 1.28$ | | [27] |
| | | 3D | $P(\delta s) \sim \delta s^{-\tau} f(\delta s/L^{\alpha})$ | 1.45 | 1.5 | [25] |
| | | 2D | $P(\delta\sigma) \sim \delta\sigma^{-\tau}$ | 1.1 | | [28] |
| Experiment | — | Metalic glass | $P(\delta s) \sim \delta s^{-\tau}$ | 1.5 | | [29] |
| | | Metalic glass | $P(\delta s) \sim \delta s^{-\tau}$ | $1.37 - 1.49$ | | [30] |
| | | Adhesive suspension | $P(s) \sim s^{-\tau}$ | 3.33 | | [31] |
| Meanfield | | | $P(n_{slip}) \sim n_{slip}^{-\tau}$ | 3/2 | | [32] |

TABLE I. Table of scaling exponents of avalanches defined through various quantities such as the stress drops ($\delta\sigma$), energy drops ($\delta E$), cluster size ($s$) of active particles, number of shear transformation activations ($S_t$), slip ($n_{slip}$) during plastic rearrangement, from numerical simulations of several systems (such as Lennard Jones (LJ), Ploy-disperse system (POLY), Stillinger Weber silicon (SW-Si)), elasto-plastic models, experiments and mean field theories.

ancies need to be further investigated. In Fig. S14(c) we show the scaled conditional distribution of the number of clusters for given avalanche size $S$ for different $S$ window to demonstrate that the distribution has a peak around its mean value.

### F. Fractal dimension and scaling relation

From the moment analysis above we see that the scaling exponents $\tau_c$ and $\beta_c$ are different in BKS-Silica and KA-BMLJ model. Assuming that the largest cluster scales with system size as $s_{max} \sim N^{\beta_c/\tau_c} \sim L^{d\beta_c/\tau_c}$, $d$ and $L$ being the spatial dimension and linear size of the system respectively, one can express the fractal dimension of the largest cluster as $d_f = d\beta_c/\tau_c$, leading to $d_f^{est} = 2.37$ for silica ($\beta_c/\tau_c \approx 0.79$) and $d_f^{est} = 1.8$ for KA-BMLJ ($\beta_c/\tau_c \approx 0.6$). We compute the fractal dimension of the largest clusters directly employing the box counting method. We divide the total system into boxes of a given mesh size and count the number of occupied boxes $N_{box}$ in which the cluster is present. In Fig. S15 we show the log-log plot of number occupied boxes $N_{box}$ against magnification $r$, the inverse of the mesh size, for BKS-Silica and KA-BMLJ. From the power-law fit of the data we obtain $d_f = 2.22 \pm 0.04$ for BKS-Silica

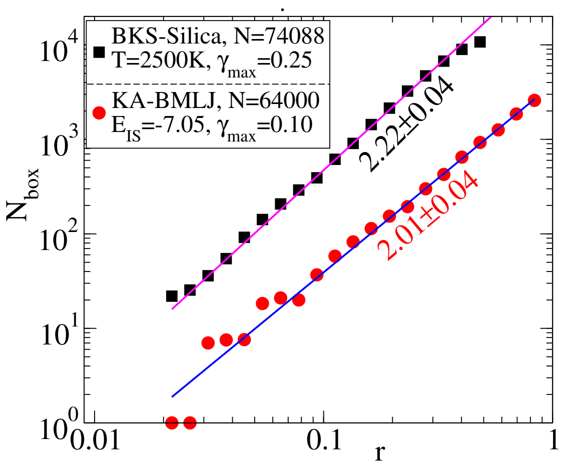


FIG. S15. The number of occupied boxes ($N_{box}$) against the magnification $r$ for BKS-Silica and KA-BMLJ model for the largest clusters. System parameters are indicated in the legends. Estimated values of the fractal dimensions for both the models are in reasonable agreement with the scaling exponents (see text).

and 2.01 ± 0.04 for KA-BMLJ. These values are found to be not exactly the same as the estimated values, but reasonably close. The fractal dimension for KA-BMLJ is consistent with the value obtained in [5] and the appearance of quasi-two dimensional shear bands [33] above yielding, and not consistent with the scaling of mean cluster size as $N^{1/3}$ [5, 34, 35]. We note, however, that the mean avalanche size previously was obtained as a ratio of second and first moments of the avalanche distribution, *i.e.*, for $m$ values for which $\alpha(m)$ does not yet show linear dependence of $m$. Employing the same ratio in the present analysis, we do obtain a $N^{1/3}$ scaling of the mean cluster size and therefore, there is no inconsistency with previous results [5].

## S-6. TETRAHEDRALITY ORDER PARAMETER

We study the orientational order parameter $q_i$ to measure the degree of tetrahedrality present in the system [36]. The orientational order parameter $q_i$ for silicon atom $i$ is given by,

$$q_i = 1 - \frac{3}{8}\sum_{j>k}\left[\cos\theta_{jik} + \frac{1}{3}\right]^2 \tag{S19}$$

where the summation is over the six possible pairs among the four closest nearest neighbors silicon atoms of $i$ and the angle $\theta_{jik}$ (the Si-Si-Si angle) formed between neighbors $j$ and $k$ and the central atom $i$. The possible values of $q_i$ lie between 0 and 1. When the atom $i$ is in the middle of a perfect tetrahedron, i.e. $\theta_{jik} \simeq 109°$, $q_i$ is equal to one. On the other hand, when the positions of the molecules are uncorrelated, the mean value is zero. The distributions of $q_i$, evaluated for the inherent structures, are presented in Fig. S16(a) for different temperatures. As expected, for low temperatures the distributions display a strong tetrahedral order, represented by the peak at $q_i \approx 0.8$. Upon increasing the temperature, the system becomes less ordered and the distribution is characterized by two populations of high and relatively low tetrahedral order. The distributions $P(q_i)$ can further be characterized by their mean and variance. In Figs. S16(b) and S16(c) we present the mean $\langle q_i\rangle_{IS}$ and variance $\langle(\partial q_i)^2\rangle_{IS} = \langle q_i^2\rangle - \langle q_i\rangle^2$ as a function of temperature. Upon lowering the temperature, the configurations display an enhanced tetrahedral order and a noticeable suppression of fluctuations.

## S-7. STATISTICS OF BOND ANGLES

To further characterize the structural change in cyclically deformed silica, following Ref. 37, we study the local bond ordering by computing atom based mean bond angle $\bar{\theta}_i$ and its standard deviation $\sigma_{\theta_i}$ defined as

$$\bar{\theta}_i = \frac{1}{n}\sum_n \theta_n^i \tag{S20}$$

$$\sigma_{\theta_i}^2 = \left(\frac{1}{n}\sum_n (\theta_n^i)^2\right) - \bar{\theta}_i^2 \tag{S21}$$

where the sum is over all possible $n$ bonds, with angles $\theta_n^i$, between the $i^{th}$ silicon atom and its nearest neighbour oxygen atoms. Note that here we consider all the nearest oxygen neighbours of a given silicon atom (not to be confused with the definition of the tetrahedral order parameter $q_i$ where we consider the four nearest neighbour silicon atoms). For convenience, we drop the subscript $i$ below. We compute the distributions of bond angle deviations $\sigma_\theta$ for different strain amplitudes and find that they exhibit clear bimodality revealing the presence of two distinct structural components in the system. In Fig. S17(a), the probability distributions $P(\sigma_\theta)$ for different strain amplitudes shows that $\sigma_\theta$ is sensitive to $\gamma_{max}$. Moreover, most of the $\sigma_\theta$ occur around $6^\circ$ with a secondary peak at $25^\circ$. With increasing strain amplitude the primary peak value decreases whereas the secondary peak value increases. We also compute the coordination number $Z_{SiO}$, the number of nearest neighbor oxygen atoms associated with each silicon atom, whose distribution is presented in Fig. S17(b). The results suggest a significant change in the fraction of 4-coordinated ($Z_{SiO} = 4$) and 5-fold ($Z_{SiO} = 5$) silicon atoms when the strain amplitude is varied. To clarify further these two types of local structures, we compute the distribution of $\sigma_\theta$ for the silicon atoms characterised by $Z_{SiO} = 4$ and $Z_{SiO} = 5$ separately. As shown in the Fig. S17(c), we

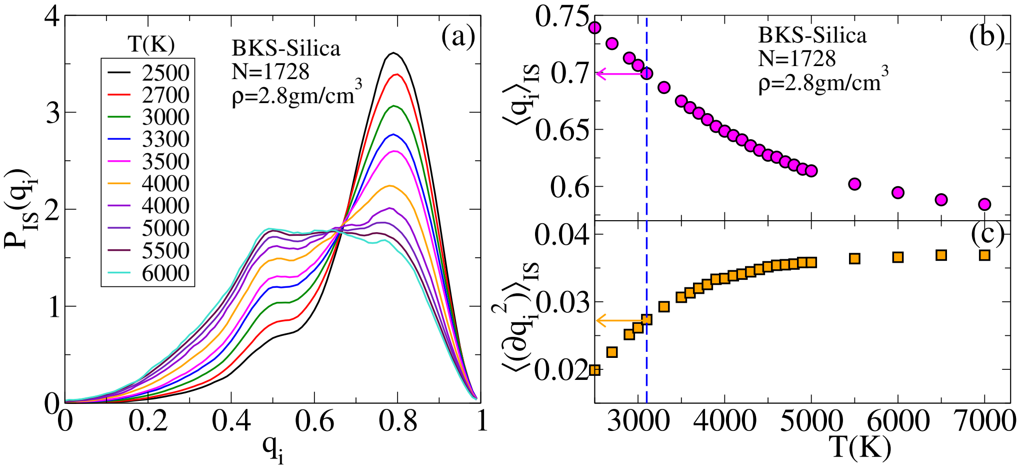


FIG. S16. (a) The distribution $P(q_i)$ of the tetrahedrality order parameter considering silicon atom positions for inherent structure configurations for different $T$, $N = 1728$. The average value (b) and variance (c) of $q_i$ as a function $T$. The vertical line is at $T_{th} = 3100K$ [4] and the arrows indicate the values of $\langle q_i \rangle_{IS}$ and $\langle (\partial q_i^2) \rangle_{IS}$ at $T_{th}$.

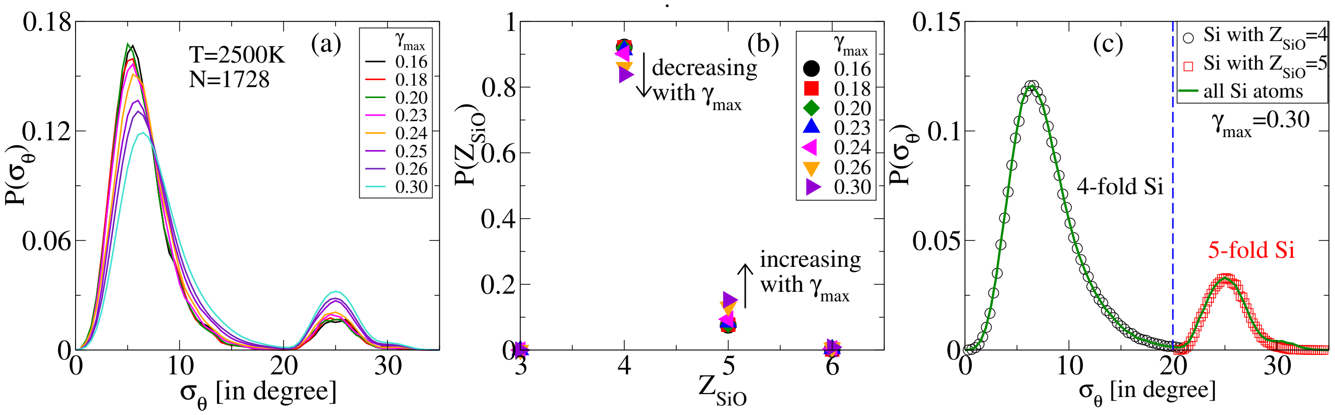


FIG. S17. (a) The distribution of the bond angle deviation $\sigma_\theta$ for stroboscopic configurations of cyclically deformed silica for several strain amplitudes. (b) Distribution of the number of nearest oxygen neighbours of silicon atoms for different $\gamma_{max}$. The probability of finding a 4-coordinated silicon atom (which has 4 oxygen neighbours) decreases and the probability of finding a 5-coordinated silicon atom increases with increasing $\gamma_{max}$, indicating more distorted tetrahedral structure. (c) Distribution of $\sigma_\theta$ for two types of silicon atoms, with $Z_{SiO} = 4$ and $Z_{SiO} = 5$. The distribution considering all the $Si$ atoms is also displayed.

find that the primary peak in $P(\sigma_\theta)$ is associated with 4-coordinated silicon atoms with small $\sigma_\theta < 20^\circ$ and with tetrahedral symmetry, whereas the secondary peak is associated with 5-coordinated silicon atoms, displaying a large bond angle deviation $\sigma_\theta > 20°$, indicating a less rigid local tetrahedral environment.

## S-8. STRAIN LOCALIZATION AND DISTORTED STRUCTURE

We evaluate the local shear strain $\epsilon_d$, as defined above, comparing configurations that are stroboscopically one cycle apart. The distributions of this quantity, $P(\epsilon_d)$, for different strain cycles are presented in Fig. S18(a). We see that the distributions exhibit a power-law for small values of $\epsilon_d$ with a cutoff around $\epsilon_d = 1.25$. To characterize the nature of the shear band, we calculate the slab-wise average local strain $\langle \epsilon_d \rangle_x$ and mean squared displacement, $MSD_x$. The system is divided into slabs of thickness $\Delta z = 3.1\mathring{A}$ along x-axis and the $\epsilon_d$ and $MSD_x$ are averaged over the atoms belonging to each slab. Interestingly, as shown in Fig. S18(b), both the quantities display a roughly Gaussian profile with a standard deviation that is related to the width of the shear band. In Fig. S18(c) we show the variation of width of the shear band against number of strain cycles. After an initial transient, as the steady state has been attained, the width fluctuates around a mean value.

Finally, we study the distribution of the standard deviation of bond angle $P(\sigma_\theta)$ and the distribution of the coordination numbers of silicon atoms, $P(Z_{SiO})$, inside the shear band (defined as those with $\epsilon_d > 1.25$), outside the shear band ($\epsilon_d < 1.25$) and for the total sys-

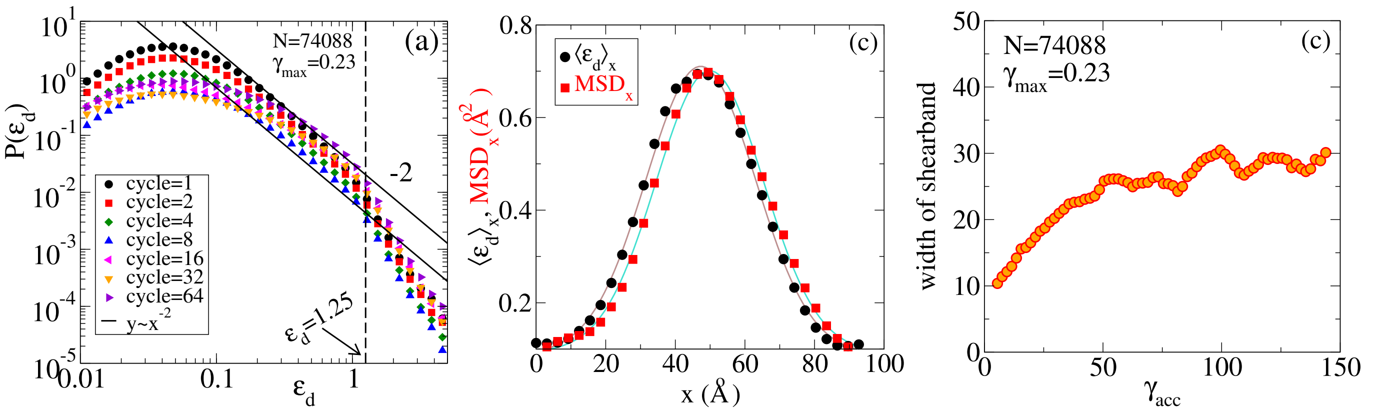


FIG. S18. (a) The distribution of $\epsilon_d$ (calculated between two consecutive zero strain stroboscopic configurations) at the end of different numbers of cycles. The vertical dashed line at $\epsilon_d \approx 1.25$ indicates the cutoff value beyond which one observes deviations from the power law. (b) Slab-wise average $MSD_x$ and local strain $\langle \epsilon_d \rangle_x$ for the same configuration of the shear band shown in the main text. Solid lines are Gaussian fits through the data points. (c) The width of the Gaussian fit against accumulated strain.

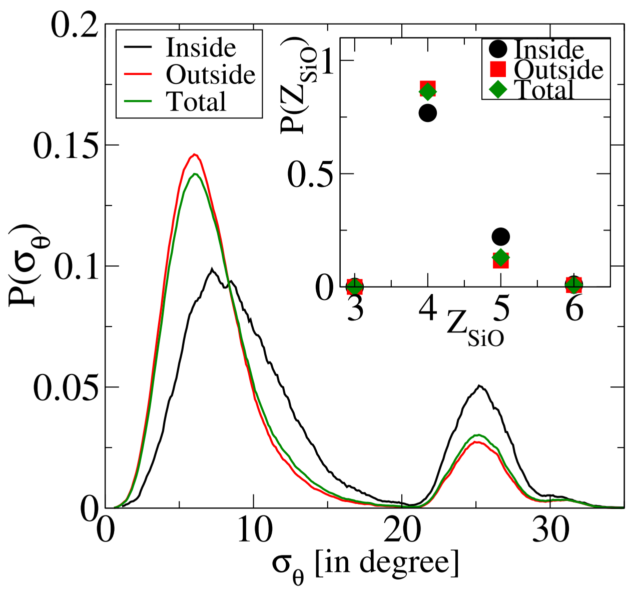


FIG. S19. The distribution of $\sigma_\theta$ computed for atoms inside the shear band, outside the shear band and for the total system for $N = 74088$ and $\gamma_{max} = 0.23$. Inset: The distribution of number of nearest oxygen neighbours of silicon atom $Z_{SiO}$. The probability of finding a 4-coordinated silicon atom (which has 4 oxygen neighbours) decreases and that of finding a 5-coordinated silicon atom increases inside the shear band, in comparison to the total system while the opposite trend is observed outside of shear band.

tem. Though this criterion does not strictly correspond to the spatial location of the shear band, as shown in Fig. 3 of the main text, atoms with $\epsilon_d > 1.25$ are indeed largely localised within the shear band. It can be seen from Fig. S19 that the distributions $P(\sigma_\theta)$ are widely different inside and outside the shear band, indicating a strong correlation between increased strain and local non-tetrahedral structure. The distributions $P(Z_{SiO})$, likewise, show that atoms with large $\epsilon_d$ correspond to lower tetrahedrality.


[1] B. W. H. van Beest, G. J. Kramer, and R. A. van Santen, "Force fields for silicas and aluminophosphates based on ab initio calculations," Phys. Rev. Lett. **64**, 1955–1958 (1990).

[2] Ivan Saika-Voivod, Francesco Sciortino, and Peter H. Poole, "Free energy and configurational entropy of liquid silica: Fragile-to-strong crossover and polyamorphism," Phys. Rev. E **69**, 041503 (2004).

[3] Davide Fiocco, Giuseppe Foffi, and Srikanth Sastry, "Oscillatory athermal quasistatic deformation of a model glass," Phys. Rev. E **88**, 020301 (2013).

[4] Himangsu Bhaumik, Giuseppe Foffi, and Srikanth Sas-

try, "The role of annealing in determining the yielding behavior of glasses under cyclic shear deformation," Proceedings of the National Academy of Sciences **118** (2021), 10.1073/pnas.2100227118.
[5] Premkumar Leishangthem, Anshul D. S. Parmar, and Srikanth Sastry, "The yielding transition in amorphous solids under oscillatory shear deformation," Nature Communications **8**, 14653 (2017), article.
[6] K. Michael Salerno and Mark O. Robbins, "Effect of inertia on sheared disordered solids: Critical scaling of avalanches in two and three dimensions," Phys. Rev. E **88**, 062206 (2013).
[7] John Douglas Eshelby, "The determination of the elastic field of an ellipsoidal inclusion, and related problems," Proceedings of the Royal Society of London. Series A. Mathematical and Physical Sciences **241**, 376–396 (1957).
[8] G. Picard, A. Ajdari, F. Lequeux, and L. Bocquet, "Elastic consequences of a single plastic event: A step towards the microscopic modeling of th e flow of yield stress fluids," European Physical Journal E **15**, 371–381 (2004).
[9] Craig E. Maloney and Anaël Lemaître, "Amorphous systems in athermal, quasistatic shear," Phys. Rev. E **74**, 016118 (2006).
[10] Anaël Lemaître and Christiane Caroli, "Rate-dependent avalanche size in athermally sheared amorphous solids," Phys. Rev. Lett. **103**, 065501 (2009).
[11] M. De Menech, A. L. Stella, and C. Tebaldi, "Rare events and breakdown of simple scaling in the abelian sandpile model," Phys. Rev. E **58**, R2677–R2680 (1998).
[12] Alessandro Chessa, H Eugene Stanley, Alessandro Vespignani, and Stefano Zapperi, "Universality in sandpiles," Physical Review E **59**, R12 (1999).
[13] Clément Le Priol, Pierre Le Doussal, and Alberto Rosso, "Spatial clustering of depinning avalanches in presence of long-range interactions," Phys. Rev. Lett. **126**, 025702 (2021).
[14] Thomas B. Schröder, Srikanth Sastry, Jeppe C. Dyre, and Sharon C. Glotzer, "Crossover to potential energy landscape dominated dynamics in a model glass-forming liquid," The Journal of Chemical Physics **112**, 9834–9840 (2000).
[15] Chen Liu, Ezequiel E Ferrero, Francesco Puosi, Jean-Louis Barrat, and Kirsten Martens, "Driving rate dependence of avalanche statistics and shapes at the yielding transition," Physical review letters **116**, 065501 (2016).
[16] Haiyan Xu, Juan Carlos Andresen, and Ido Regev, "Yielding in an amorphous solid subject to constant stress at finite temperatures," Phys. Rev. E **103**, 052604 (2021).
[17] Norihiro Oyama, Hideyuki Mizuno, and Atsushi Ikeda, "Unified view of avalanche criticality in sheared glasses," (2020), arXiv:2009.02635 [cond-mat.soft].
[18] Gaurav Prakash Shrivastav, Pinaki Chaudhuri, and Jürgen Horbach, "Yielding of glass under shear: A directed percolation transition precedes shear-band formation," Phys. Rev. E **94**, 042605 (2016).
[19] Tomoaki Niiyama, Masato Wakeda, Tomotsugu Shimokawa, and Shigenobu Ogata, "Structural relaxation affecting shear-transformation avalanches in metallic glasses," Phys. Rev. E **100**, 043002 (2019).
[20] Misaki Ozawa, Ludovic Berthier, Giulio Biroli, Alberto Rosso, and Gilles Tarjus, "Random critical point separates brittle and ductile yielding transitions in amorphous materials," Proceedings of the National Academy of Sciences **115**, 6656–6661 (2018).
[21] Michael J. Demkowicz and Ali S. Argon, "Autocatalytic avalanches of unit inelastic shearing events are the mechanism of plastic deformation in amorphous silicon," Phys. Rev. B **72**, 245206 (2005).
[22] Alexandra E. Lagogianni, Chen Liu, Kirsten Martens, and Konrad Samwer, "Plastic avalanches in the so-called elastic regime of metallic glasses," The European Physical Journal B **91**, 104 (2018).
[23] Ido Regev, John Weber, Charles Reichhardt, Karin A Dahmen, and Turab Lookman, "Reversibility and criticality in amorphous solids," Nature Communications **6**, 8805–8805 (2015).
[24] Mehdi Talamali, Viljo Petäjä, Damien Vandembroucq, and Stéphane Roux, "Avalanches, precursors, and finite-size fluctuations in a mesoscopic model of amorphous plasticity," Phys. Rev. E **84**, 016115 (2011).
[25] Jie Lin, Edan Lerner, Alberto Rosso, and Matthieu Wyart, "Scaling description of the yielding transition in soft amorphous solids at zero temperature," Proceedings of the National Academy of Sciences **111**, 14382–14387 (2014), https://www.pnas.org/content/111/40/14382.full.pdf.
[26] Jie Lin, Thomas Gueudré, Alberto Rosso, and Matthieu Wyart, "Criticality in the approach to failure in amorphous solids," Phys. Rev. Lett. **115**, 168001 (2015).
[27] Zoe Budrikis, David Fernandez Castellanos, Stefan Sandfeld, Michael Zaiser, and Stefano Zapperi, "Universal features of amorphous plasticity," Nature Communications **8**, 15928 (2017).
[28] E. A. Jagla, "Avalanche-size distributions in mean-field plastic yielding models," Phys. Rev. E **92**, 042135 (2015).
[29] James Antonaglia, Wendelin J. Wright, Xiaojun Gu, Rachel R. Byer, Todd C. Hufnagel, Michael LeBlanc, Jonathan T. Uhl, and Karin A. Dahmen, "Bulk metallic glasses deform via slip avalanches," Phys. Rev. Lett. **112**, 155501 (2014).
[30] B. A. Sun, H. B. Yu, W. Jiao, H. Y. Bai, D. Q. Zhao, and W. H. Wang, "Plasticity of ductile metallic glasses: A self-organized critical state," Phys. Rev. Lett. **105**, 035501 (2010).
[31] Zhouyang Ge, Raffaella Martone, Luca Brandt, and Mario Minale, "Irreversibility and rate dependence in sheared adhesive suspensions," (2021), arXiv:2106.14341 [cond-mat.soft].
[32] Karin A. Dahmen, Yehuda Ben-Zion, and Jonathan T. Uhl, "A simple analytic theory for the statistics of avalanches in sheared granular materials," Nature Physics **7**, 554–557 (2011).
[33] Anshul D. S. Parmar, Saurabh Kumar, and Srikanth Sastry, "Strain localization above the yielding point in cyclically deformed glasses," Phys. Rev. X **9**, 021018 (2019).
[34] Edan Lerner and Itamar Procaccia, "Locality and nonlocality in elastoplastic responses of amorphous solids," Phys. Rev. E **79**, 066109 (2009).
[35] Smarajit Karmakar, Edan Lerner, and Itamar Procaccia, "Statistical physics of the yielding transition in amorphous solids," Phys. Rev. E **82**, 055103 (2010).
[36] M. Scott Shell, Pablo G. Debenedetti, and Athanassios Z. Panagiotopoulos, "Molecular structural order and anomalies in liquid silica," Phys. Rev. E **66**, 011202 (2002).
[37] M. J. Demkowicz and A. S. Argon, "High-density liq-

uidlike component facilitates plastic flow in a model amorphous silicon system," Phys. Rev. Lett. **93**, 025505 (2004).
